# Supplementary material for: Raman study of the structural transition in LiVO$_2$
Source: arXiv:2407.08426 source file (2024-07-11)
Supplement: Supplementary file 1 [file Supp.pdf]

# Raman study of the structural transition in $LiVO_2$

Yuri S. Ponosov,[1] Evgenia V. Komleva,[1, 2] Elizaveta A.Pankrushina,[3]
Haohang Xu,[4] Yu Sui,[4] and Sergey V. Streltsov[1, 2]

[1]Institute of Metal Physics, Ural Branch of the Russian Academy of Sciences, Ekaterinburg 620137, Russia

[2]Department of theoretical physics and applied mathematics,
Ural Federal University, Ekaterinburg 620002, Russia

[3]Laboratory of Arctic Mineralogy and Material Sciences, Kola Science Centre, Russian Academy of Sciences, Apatity 184209, Russia

[4] Harbin Institute of Technology, China

Temperature dependences of Raman spectra obtained for the second and third crystals.

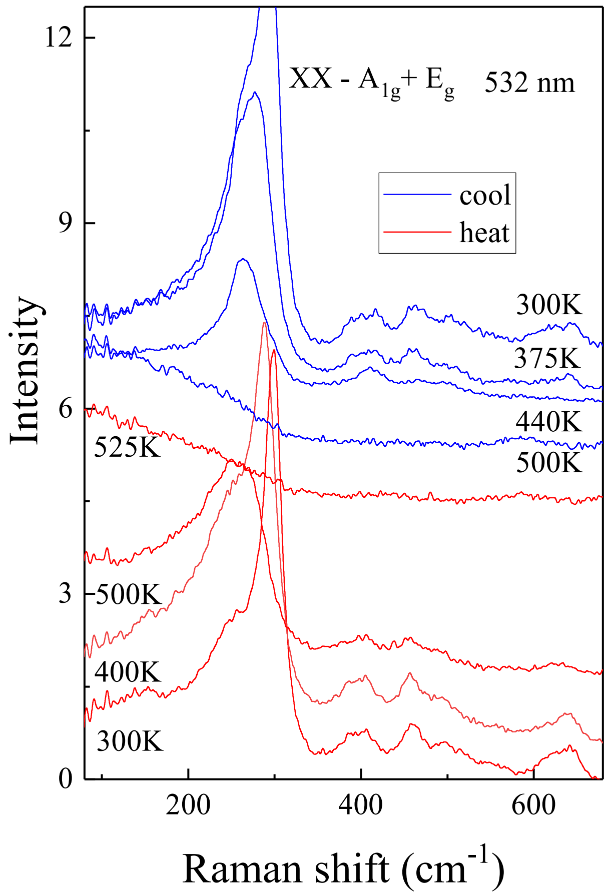


Fig.S1. Temperature dependent Raman spectra in XX scattering geometry measured in the heat-cool cycle of the second crystal.

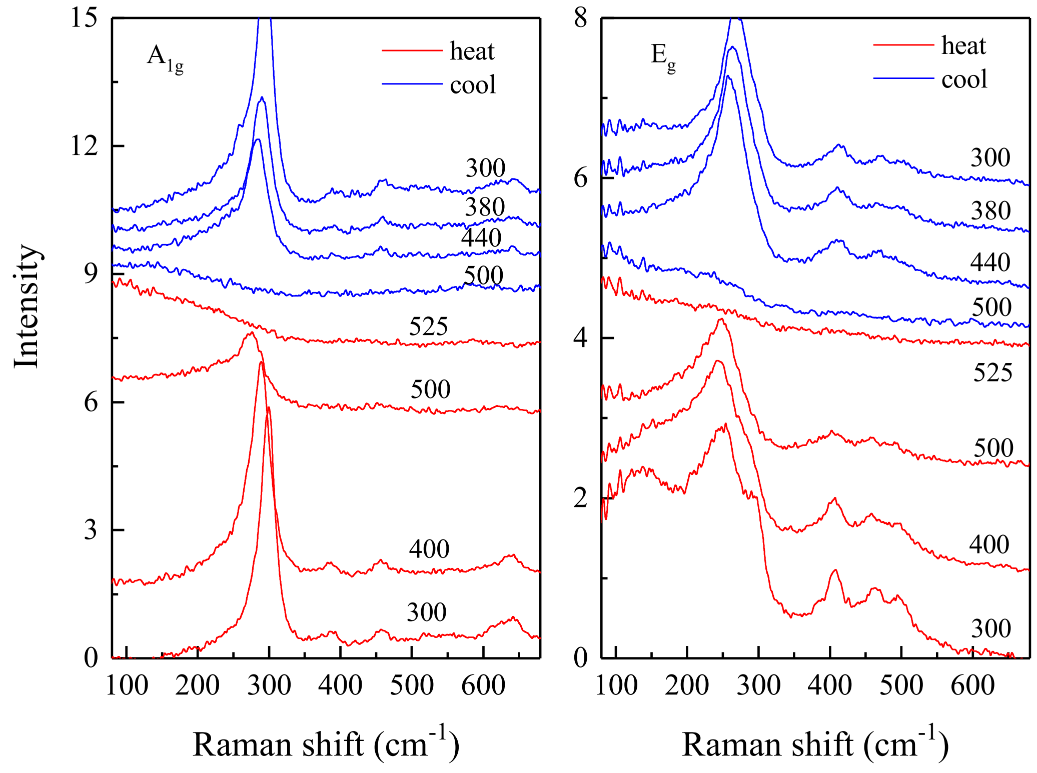


Fig.S2. Temperature dependent Raman spectra in both scattering geometries measured in the heat-cool cycle of the second crystal.

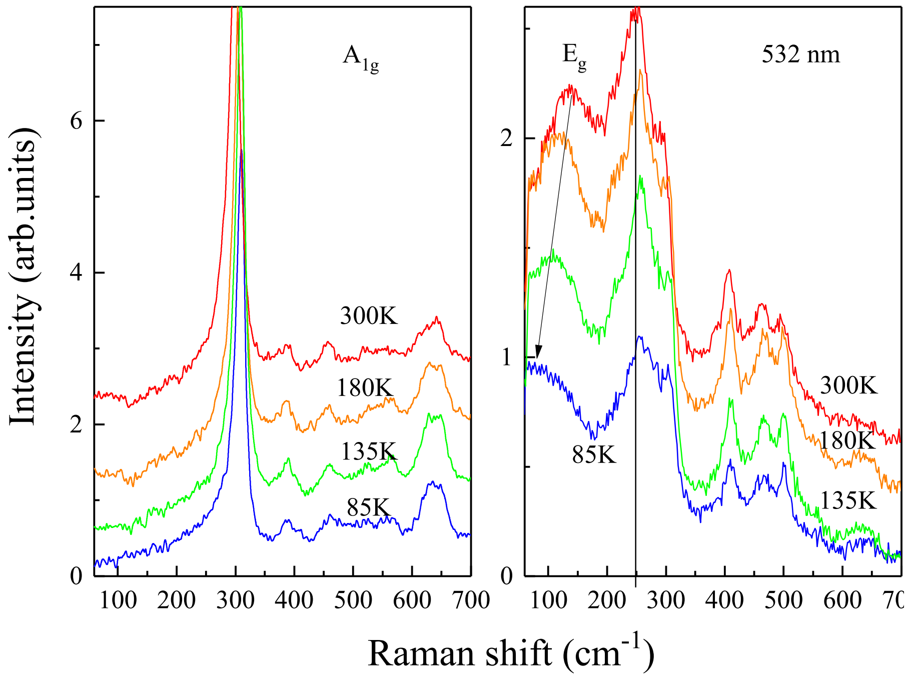


Fig.S3. Low temperature $A_{1g}$ and $E_g$ Raman spectra of the second $LiVO_2$ crystal.

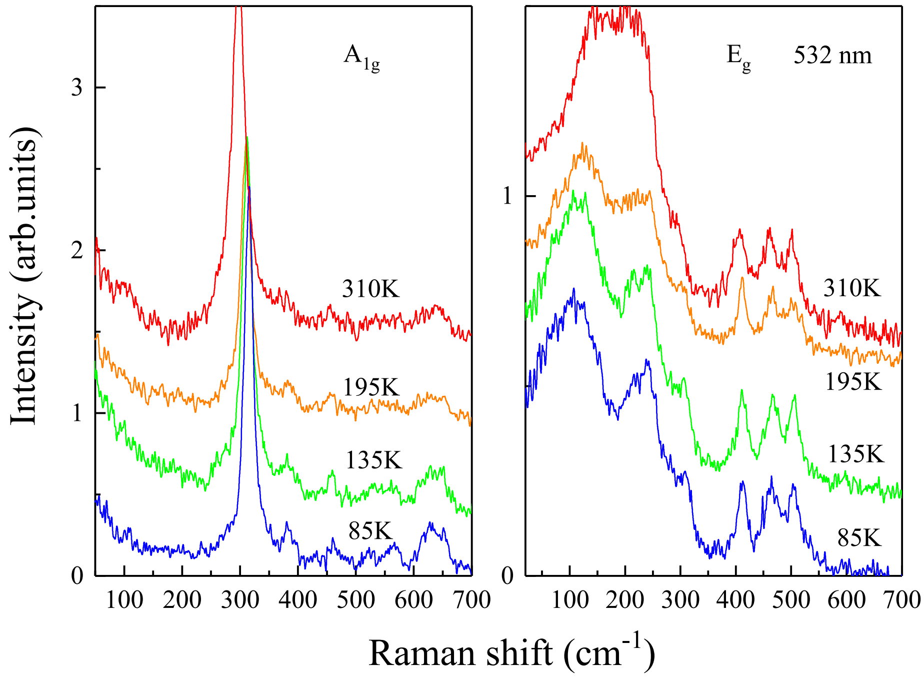


Fig.S4. Low temperature $A_{1g}$ and $E_g$ Raman spectra of the third $LiVO_2$ crystal.
